# Supplementary material for: Multi-dimensional Test Design
Source: arXiv:2502.12264 source file (2025-02-17)
Supplement: Supplementary file 1 [file A_ex_non_parallel_test.tex]

\section{An example with non-parallel tests}\label{appendix: counter ex}
In the following example, we show that for some distributions, the optimal fixed-order mechanism in the manipulation setting and program \ref{max qualified} uses a classifier with a boundary not parallel to the qualified region boundary.

Let the qualified region be the intersection of two classifiers $\classifier_A$ and $\classifier_B$. 
The angle between $\classifier_A$ and $\classifier_B$ is $60^\circ$\xqcomment{we want to show it for every $\theta$}.
Let $O$ be the intersection point of their boundaries. 
Let $\classifier_i^+ $ be the half plane obtained by shifting $\classifier_i$ along its normal vector $\weights_i$ by a distance of $1/\eta$.
Let $O^+$ be the intersection point of the boundary lines of $\classifier_A^+ $ and $\classifier_B^+ $.
Let $\tilde\classifier_A$ be the half plane obtained by rotating $\classifier_A^+ $ around point $O^+$ towards $\classifier_B^+ $ until the boundary line is exactly the angle bisector of $\classifier_A^+ $ and $\classifier_B^+$, which means the boundary of $\tilde \classifier_A$ goes through $O$.
See \cref{fig:non-parallel tests} for an illustration.
Consider the fixed order mechanism $(\classifier_A^+,\classifier_B^+,1)$ and the fixed order mechanism $(\tilde\classifier_A,\classifier_B^+,1)$.

We now show that the fixed-order mechanism $(\tilde\classifier_A,\classifier_B^+,1)$ with non-parallel classifiers is better than the fixed-order mechanism $(\classifier_A^+,\classifier_B^+,1)$ for certain distribution. 

Let $A$ be the intersection of boundaries of $\classifier_B$ and $\classifier_A^+$. Let $B$ be the intersection of boundaries of $\classifier_A$ and $\classifier_B^+$.

By the characterization of the fixed-order mechanism, all attributes in the triangle $\Updelta \text{OAB}$ are admitted by the fixed order mechanism $(\tilde\classifier_A,\classifier_B^+,1)$ but are not admitted by the fixed order mechanism $(\classifier_A^+,\classifier_B^+,1)$. 
Consider a line parallel to the boundary of $\tilde\classifier_A$ and has distance $1/\eta$ to it. 
On another, all attributes in the area $ECD$ are admitted by the fixed order mechanism $(\classifier_A^+,\classifier_B^+,1)$ but are not admitted by the fixed order mechanism $(\classifier_A^+,\classifier_B^+,1)$.

\begin{figure}
\centering
\begin{tikzpicture}[xscale=5,yscale=5]

\draw [thick] (-0.25,{-0.25/tan(30)}) -- (-0.25,0.8);
\draw [domain=-0.25:0.8, thick] plot (\x, {tan(30)*\x-0.25/cos( 30)});
\node [below] at (-0.25, {tan(30)*(-0.25)-0.25/cos( 30)} ) {$O$};

\node [above] at (-0.25, 0.8 ) {$\classifier_B$};
\node [above] at (0.8, {tan(30)*0.8-0.25/cos( 30)} ) {$\classifier_A$};
\node [below] at (0.8, {tan(30)*0.8-0.25/cos( 30)} ) {$D$};
% \draw [domain=-0.5:0.25, thick] plot (\x, {-tan(60)*(\x+0.25/cos( 30))});

\draw [thick, blue] (0,0) -- (0,0.8);
\draw [domain=-0.25:0.7, thick, blue] plot (\x, {tan(30)*\x});
\node [above, blue] at (0, 0.8 ) {$\classifier_B^+$};
\node [right, blue] at (0.7, {tan(30)*0.7} ) {$\classifier_A^+$};
\draw [domain=-0.25:0, blue] plot (\x, {-tan(30)*\x-0.5*tan(30)});
\node [right] at (0, {-0.5*tan(30)} ) {$B$};
\node [left] at (-0.25, {tan(30)*0.25-0.5*tan(30)}) {$A$};

\draw [domain=-0.25:0.4, thick, red] plot (\x, {tan(60)*\x});
\node [above, red] at (0.4, {tan(60)*0.4} ) {$\tilde\classifier_A$};

\draw [domain={0.25*sin(60)}:0.6, densely dashed, red] plot (\x, {tan(60)*\x-0.25/cos(60)});
\node[above] at (0.6, {tan(60)*0.6-0.25/cos(60)}) {$E$};

\draw [ red] (0,0) -- ({0.25*sin(60)},{-0.25*cos(60)});
\draw[red] ({0.25*sin(60)},{-0.25*cos(60)}) arc (-30:-60:0.25);
\draw [ red] (-0.25,0) -- (0,0);
\draw [ red] (-0.25,0) -- (-0.25,{-0.25/tan(30)});
\draw [ red] ({0.25*sin(30)},{-0.25*cos(30)}) -- (-0.25,{-0.25/tan(30)});
\node[right] at  ({0.25*sin(30)},{-0.25*cos(30)}) {$C$};

\node [right] at (-0.25,0.76 ) {$+$};
\node [left] at (0.8, {tan(30)*0.8-0.25/cos( 30)}) {$+$};
\node [left, red] at (0.4, {tan(60)*0.4}) {$+$};

\fill [orange!60,nearly transparent]  (-0.25,{-0.25/tan(30)}) -- (-0.25,{-0.25*tan(30)}) -- (0,{-0.5*tan(30)}) -- cycle;
\node [above, thick, orange] at (0, {-0.25/tan(30)}) {gain};

\fill [purple!60,nearly transparent]  (0.6,{tan(60)*0.6-0.25/cos(60)}) -- ({(0.25/cos(60)-0.25/cos(30))/(tan(60)-tan(30))},{tan(30)*(0.25/cos(60)-0.25/cos(30))/(tan(60)-tan(30))-0.25/cos( 30)}) -- (0.8, {tan(30)*0.8-0.25/cos( 30)}) -- cycle;
\node [above, thick, purple] at (0.68, {tan(30)*0.7}) {loss};

\end{tikzpicture}
\caption{An example of non-parallel tests} \label{fig:non-parallel tests}  
% \rule{0in}{1.2em}$^\dag$\scriptsize Consider 
\end{figure}
